# Supplementary material for: A semantic embedding space based on large language models for modelling human beliefs
Source: arXiv:2408.07237 source file (2025-06-06)
Supplement: Supplementary file 1 [file Supporting_information.pdf]

# Supporting Information for

## Neural embedding of beliefs reveals the role of relative dissonance in human decision-making

Byunghwee Lee, Rachith Aiyappa, Yong-Yeol Ahn, Haewoon Kwak, Jisun An

Jisun An, Haewoon Kwak

E-mail: Jisunan@iu.edu, hwkwak@iu.edu

### This PDF file includes:

Figs. S1 to S10

Tables S1 to S4

SI References

## Contents

|          |                                                                    |          |
|----------|--------------------------------------------------------------------|----------|
| <b>1</b> | <b>Basic statistics</b>                                            | <b>2</b> |
| <b>2</b> | <b>Data pre-processing</b>                                         | <b>2</b> |
| <b>3</b> | <b>Evaluation of template variability on belief embeddings</b>     | <b>3</b> |
| <b>4</b> | <b>Belief Embedding</b>                                            | <b>4</b> |
| A        | Belief Embedding in UMAP . . . . .                                 | 4        |
| B        | User embedding of the base S-BERT model . . . . .                  | 5        |
| <b>5</b> | <b>Predicting user beliefs on new debates</b>                      | <b>5</b> |
| A        | Average accuracy for belief prediction over user history . . . . . | 5        |
| B        | Average accuracy for belief prediction over $d_{avg}$ . . . . .    | 5        |

## 1. Basic statistics

The Debate.org (DDO) dataset (1, 2) utilized in this study comprises a corpus of 78,376 debates, spanning from October 15, 2007, to September 19, 2018. The pre-processing described in the Methods section of the main manuscript resulted in a curated subset of 65,861 debates with 59,986 unique debate titles. Fig. S1 shows the number of debates and user participation, in roles such as debaters and voters, over time during the period under consideration.

Fig. S2 demonstrates the basic statistics of user participation. The distributions of number of debates in which users participated by voting follows a heavy-tailed distribution (Fig. S2a). The heterogeneity in user participation indicates that most users participate in a small number of debates, while a smaller but significant number of active users are involved in many debates. The number of voters per debate also follows a heavy-tailed distribution (Fig. S2b), demonstrating that most debates have very few voters, but there are still some significant number of debates where hundreds of people participated into voting.

## 2. Data pre-processing

In the pre-processing stage, we filtered unsuitable debate titles using GPT-4, one of the most advanced and reliable artificial intelligence language model (3). We designed a prompt to ask GPT-4 to determine whether a given statement (debate title) can be considered a human belief. Fig. S3 shows a sample prompt given to GPT-4. Among 68,900 unique debate titles, GPT-4 classified 8,914 as unsuitable for consideration as belief statements.

To assess the consistency of GPT-4’s classification results with human annotations, we compared its

classifications of 50 randomly sampled debate titles with those determined by three human annotators. We equally sampled 25 titles from each category of ‘True’ and ‘False’, as classified by GPT-4, to ensure balanced representation. We then asked the three annotators to classify the 50 debate titles into two categories—those considered to reflect human belief and those that are not—using questions similar to those used for GPT-4’s categorization. The sampled debate titles are listed in Table S1.

GPT-4’s classifications showed an 88% agreement rate with the majority vote of the human annotators (Fig. S4a and b), suggesting strong consistency between GPT-4’s classifications and human consensus in identifying belief statements. The inter-annotator reliability, measured by Fleiss’ Kappa was 0.866, indicating a high level of agreement among the human annotators (Fig. S4c).

### 3. Evaluation of template variability on belief embeddings

In this study, we consider the combination of a user’s vote position (Pro/Con) and the debate title as belief statements. To express these belief statements in a sentence, we used template phrases such as, ‘I agree/disagree with the following:’ followed by the debate title. We tested whether a belief space trained using one template is robust to variations introduced by alternative templates.

We employed S-BERT, fine-tuned with belief statements generated using the original template (“I agree/disagree with the following: ”). To test if the model behaves similarly for other templates, we rephrased belief statements using three alternative templates as shown in Table S2. Then we conducted triplet evaluation tasks, which involve assessing whether positive belief pairs were closer in Euclidean distance than negative pairs. We calculated the triplet evaluation accuracy for both the original template and the rephrased templates using the S-BERT fine-tuned with the original template.

Table S3 demonstrates the triplet evaluation accuracy measured for the belief set with the original template and for the same belief set rephrased with the alternative templates. Despite variations in template phrasing, the triplet evaluation accuracy remained similar across different templates, indicating that the model could effectively distinguish between positive and negative relations of belief pairs.

We also visualized the belief embeddings in the first two principal component (PC) spaces for three example keywords: ‘God,’ ‘Abortion,’ and ‘Gay’ to determine if the distribution of belief embeddings remains consistent across different templates. Fig. S5 illustrates that the embeddings for the three keywords exhibit similar distributions across different template phrases. The panels in the first column demonstrate embeddings generated using the original template, while the other columns display embeddings for the

same beliefs but rephrased with three alternative templates. The bimodal distribution of belief embeddings was preserved across different template choices, suggesting the model's robustness to template variability.

The results suggest that the belief space, fine-tuned with the original template, remains effective and consistent even when alternative templates are used. This demonstrates the model's robustness and reliability in handling different phrasings of belief statements.

## 4. Belief Embedding

**A. Belief Embedding in UMAP.** In addition to the principal component analysis of belief space, we also employ Uniform Manifold Approximation and Projection (UMAP) (4), an advanced dimensionality reduction technique based on manifold learning and topological data analysis, to explore how our model transforms the structure of belief space. UMAP is well-suited for visualizing the belief space as it effectively reduces the complexity of the high dimensional belief space while retaining significant relational information among beliefs.

To illustrate how beliefs on various topics are distributed in the belief space, we sampled ten representative belief groups, each consisting of a unique set of keywords. For instance, within the DDO dataset, there are 5,324 distinct beliefs including the keyword 'God (god)' and 908 beliefs that consist of 'Abortion'. Fig. S6a presents the clustering of beliefs related to distinct keywords in the UMAP space of the belief embedding space.

While the entire set of beliefs (Fig. S6b) exhibit an evenly spread distribution across a broad region, the density plots for beliefs related to specific keywords, such as 'God' and 'Abortion', reveal highly polarized distributions with two distinct clusters (Fig. S6c). These patterns suggest that beliefs regarding these topics are grouped into two clusters with contrasting opinions, reflecting the existing political polarization on various social issues.

In addition, the proximity of clusters of beliefs related to different keywords, reveals the interconnections between two belief groups. For instance, beliefs favoring the existence of God and opposing abortion are predominantly found on the far left side of the UMAP space, whereas beliefs that reject the existence of God/god and support abortion rights tend to cluster on the far right (Fig. S6a). This indicates beliefs that supports God/god are more closely related with those beliefs that are against abortion. Similarly, beliefs related to 'Gay and gay marriage,' 'Prostitution,' 'Global warming,' and 'Evolution and Darwin' exhibit two dense, distant clusters in the belief space (Fig. S6c).



**B. User embedding of the base S-BERT model.** We obtained user embeddings for individual users in the belief space by averaging all belief vectors belonging to each user. This allows us to represent users in the same belief space with their beliefs.

To validate whether the resulting user representations exhibit any patterns of polarization, we visually mapped users based on their self-reported survey responses. In the DDO, users can express their opinions on major social issues through a pre-survey, distinct from their debate participation. This survey includes specifying their supporting political parties, religious ideologies, and positions on 48 key social issues, known as ‘big issues.’ These issues encompass a range of controversial topics such as ‘abortion,’ ‘drug legalization,’ ‘gun control,’ and others.

Fig. 3 in the main manuscript visualizes users in the belief space, color-coding them based on their pre-survey results on the big issues. The distribution of user embedding produced using the fine-tuned S-BERT model exhibits a clear separation of user groups with different positions on big issues in the belief space. In contrast, the user embeddings generated using the base S-BERT model do not show such clear separation of users (Fig. S7).

## 5. Predicting user beliefs on new debates

In the downstream task, we conducted a binary belief classification aimed at predicting an individual’s voting position (PRO or CON) in new debates. We divided the entire set of debates into an 8:2 ratio and evaluated the model’s performance using 5-fold cross-validation. We considered users who appeared at least once in both the train and test sets. Table S4 summarizes the basic statistics of the train and test datasets.

**A. Average accuracy for belief prediction over user history.** Fig. S9 shows the performance of the belief prediction downstream task as a function of the length of user voting history,  $L_v$ . As the users’ voting records increase, their beliefs tend to be more accurately predicted.

**B. Average accuracy for belief prediction over  $d_{\text{avg}}$ .** we measured how belief prediction accuracy changes depending on the average distance between the user and two conflicting beliefs for a given debate,  $d_{\text{avg}}$ . As  $d_{\text{avg}}$  increases, the accuracy tends to level off at 0.5, akin to random choice baseline. Fig. S10 shows how average accuracy for belief prediction changes with  $d_{\text{avg}}$ .

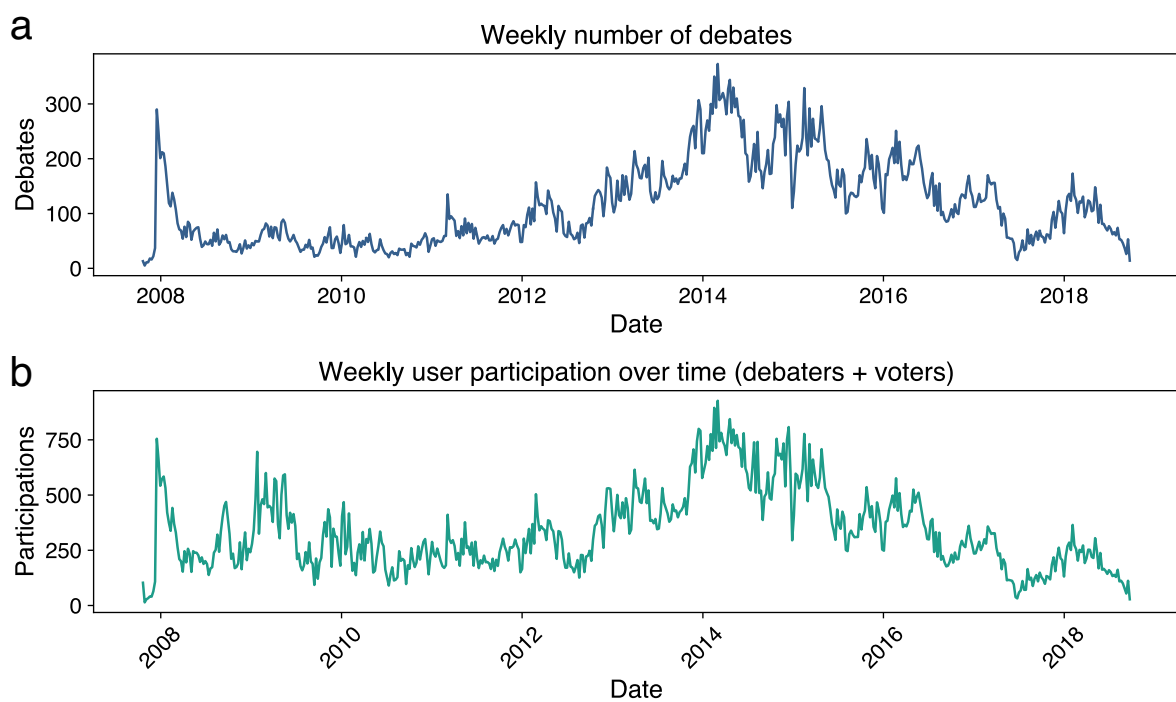

**Fig. S1.** (a) Weekly number of debates over time. The curated DDO dataset utilized in this study comprises a corpus of 65,861 debates, spanning from October 15, 2007, to September 19, 2018. (b) Weekly number of participants (both debaters and voters) in DDO dataset.

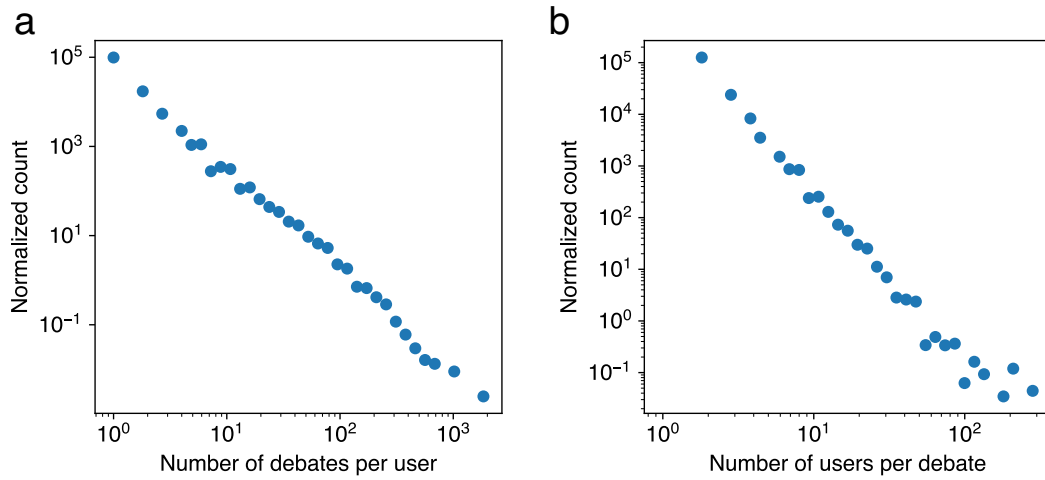

**Fig. S2.** Distribution of the number of debates participated in per user (a) and user participation per debate (b), where the Y-axes represent the log-binned distributions of normalized counts. Both distributions exhibit heavy-tailed characteristics, implying that most users participate in a small number of debates, while a smaller but significant number of users are involved in many debates. Similarly, there are a smaller but significant number of debates in which many users participated.

**System role** You are an annotator tasked with determining whether a given statement can be considered a human belief. Answer '1' if the statement can be considered a belief statement, and '0' if it cannot be considered a belief statement.

**Constraint** You must provide an answer and give answer in comma separated list.

**Examples** Here is an example.

example statements:

A complete gun ban in the United States

A Completely Omnipotent Being Cannot Logically Exist

A Comprehensive Immigration Reform is key to our Economy and one should be issued  
a computer gives a headache

A conclusion to the art of communication

answer:

1, 1, 1, 1, 0

**Context** Debate title 1  
Debate title 2  
...  
Debate title 10

**Fig. S3.** Prompt used to filter unsuitable debate titles using GPT-4. We constructed a prompt that instructs the model to assess whether each debate title can be considered human belief.

**Table S1. 50 sample debate titles with corresponding GPT-4 classification results (1: title can be considered a human belief, 0: otherwise). These titles were used for comparison with human annotators' results.**

|    | Debate title                                                                                        | GPT-4 label |
|----|-----------------------------------------------------------------------------------------------------|-------------|
| 1  | In the United States, Minor Jail Time Ought to be Replaced with Significant Rehabilitation.         | 1           |
| 2  | should gay marriage be legal?                                                                       | 0           |
| 3  | Stand your ground.                                                                                  | 0           |
| 4  | Prove that the god according to the bible loves and cares for/ about the ENTIRE human race          | 0           |
| 5  | Do or Do Not there is no try. Do you Agree?                                                         | 1           |
| 6  | Batman (pro) VS Deadpool (con)                                                                      | 0           |
| 7  | CBA Child Abuse                                                                                     | 0           |
| 8  | Design Your Prison                                                                                  | 0           |
| 9  | Eugenics                                                                                            | 0           |
| 10 | Is rap/hip-hop music "bad"?                                                                         | 1           |
| 11 | The death penalty, is it A- Morally Right and B- Logically Right                                    | 1           |
| 12 | Government should get out of the marriage business                                                  | 1           |
| 13 | Mars colony                                                                                         | 0           |
| 14 | Since good secure more happiness, we should live good.                                              | 1           |
| 15 | Metal Detectors in Schools?                                                                         | 1           |
| 16 | The United States needs Universal Healthcare.                                                       | 1           |
| 17 | Give me riddles                                                                                     | 0           |
| 18 | New Lyrical Challenge                                                                               | 0           |
| 19 | Irish vs. British rap battle                                                                        | 0           |
| 20 | Anarcho-capitalism is the right form of government                                                  | 1           |
| 21 | Beauty is only skin deep.                                                                           | 1           |
| 22 | Chemical sterilization for non-custodial parents of 2 or more children that don't pay child support | 1           |
| 23 | The Patriots undefeated season should have an asterisk on it.                                       | 1           |
| 24 | Riddle of Epicurus                                                                                  | 0           |
| 25 | Agriculture vs. Population                                                                          | 0           |
| 26 | The Qur'an is not the truth, Jesus is God                                                           | 1           |
| 27 | fasion                                                                                              | 0           |
| 28 | Surrogate Mothers                                                                                   | 0           |
| 29 | Stateless society                                                                                   | 0           |
| 30 | Should Jerusalem be a Jewish territory                                                              | 1           |
| 31 | Were classical composers gay?                                                                       | 0           |
| 32 | Should studens be forced to take an extra curricular activity?                                      | 1           |
| 33 | Dr. Ben Carson or Hillary Clinton?                                                                  | 0           |
| 34 | tom brady is better than peyton manning                                                             | 1           |
| 35 | Resolved: The term "terrorist" is discriminatory towards muslim United States citizen's.            | 1           |
| 36 | Any government attempts to bail out homeowners in foreclosure are wrong and unfair to tax payers.   | 1           |
| 37 | High school, 8th grade and off into a big school where you stay there from sept. 1 to june 1st      | 0           |
| 38 | Interactive novels                                                                                  | 0           |
| 39 | Should pooping be Illegal?                                                                          | 1           |
| 40 | Random Poetry Battle                                                                                | 0           |
| 41 | 7-Day Cycle of Masturbation Abstinence Helps Attract Women                                          | 1           |
| 42 | Religion is a modern day myth.                                                                      | 1           |
| 43 | Terrorism Can Be Justified                                                                          | 1           |
| 44 | LD Debates                                                                                          | 0           |
| 45 | Should gay marriage be allowed???                                                                   | 1           |
| 46 | Should we, as christians, Doubt the Bible sometimes?                                                | 1           |
| 47 | Just for fun! 1+1=2                                                                                 | 0           |
| 48 | Nuclear weapons are a necessary evil, and disarmament will only bring worse problems.               | 1           |
| 49 | Best way to murder somebody without getting caught                                                  | 0           |
| 50 | Nuclear power.                                                                                      | 0           |

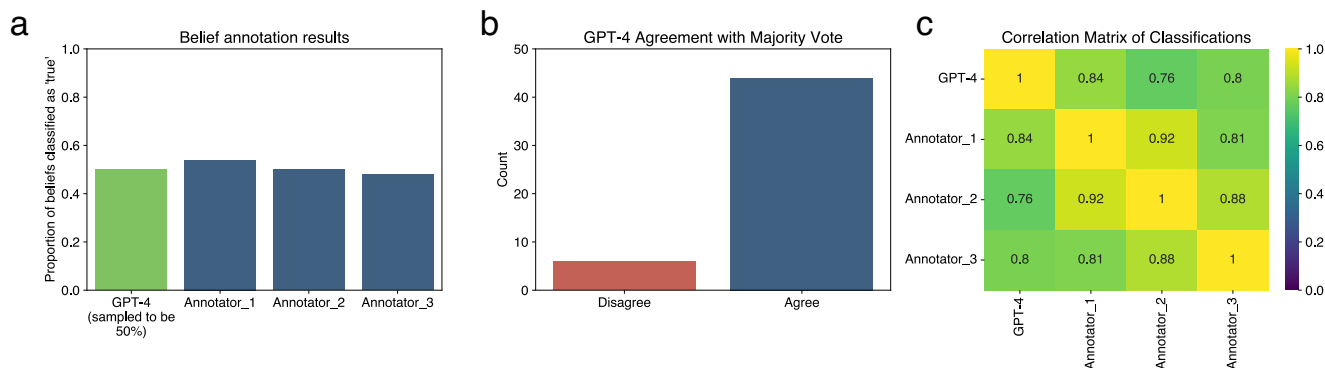

**Fig. S4.** Validation of the belief filtering process using GPT-4 by comparison with human annotation. We sampled 25 titles from each category of 'True' and 'False,' as classified by GPT-4. Then we asked three human annotators to classify the 50 debate titles into two categories: those that are considered human belief and those that are not. (a) Proportions of beliefs classified as 'True' by each annotator. Similar outcomes from annotators suggest that there is a general agreement on classification results among them. (b) The number of agreements and disagreements between GPT-4's classifications and the majority vote from human annotators. The high count of agreements (44 out of 50, 88% agreement rate) emphasizes GPT-4's alignment with human consensus. (c) correlation matrix of classifications by human annotators. Strong positive correlations indicate consistent agreement between annotators on the classification of statements as beliefs or non-beliefs.

**Table S2.** For a given debate title, we used template phrases to express Pro and Con stances. The table shows the original template phrases used for fine-tuning the model, along with three types of alternative phrases for each stance.

| Stance | Original template phrases         | Alternative phrases                                                                                                                                        |
|--------|-----------------------------------|------------------------------------------------------------------------------------------------------------------------------------------------------------|
| Pro    | "I agree with the following: "    | Type 1: "I support the following statement: "<br>Type 2: "I am in accord with the following: "<br>Type 3: "I am aligned with the following points: "       |
| Con    | "I disagree with the following: " | Type 1: "I do not support the following statement: "<br>Type 2: "I am in discord with the following: "<br>Type 3: "I am opposed to the following points: " |

**Table S3.** Triplet evaluation tested with three alternative template phrases. For given triplets, the evaluation task examines whether the positive pairs are closer in Euclidean distance than the negative pairs. Higher accuracy indicates that the model clearly distinguishes positive and negative relations of belief pairs. The first row depicts the original triplet evaluation. The other three rows demonstrate the triplet evaluation accuracy measured using the same training and test triplets but with alternative template phrases for Pro and Con stances. We tried three different types of templates, as shown in Table S2. The triplet evaluation accuracy remained similar under different choices of templates.

| <b>Template phrases</b> | <b>Triplet evaluation accuracy<br/>- Train set (Mean &amp; Std.)</b> | <b>Triplet evaluation accuracy<br/>- Test set (Mean &amp; Std.)</b> |
|-------------------------|----------------------------------------------------------------------|---------------------------------------------------------------------|
| Original                | 0.977 (0.003)                                                        | 0.675 (0.015)                                                       |
| Type 1                  | 0.972 (0.004)                                                        | 0.673 (0.017)                                                       |
| Type 2                  | 0.968 (0.003)                                                        | 0.672 (0.016)                                                       |
| Type 3                  | 0.922 (0.010)                                                        | 0.677 (0.013)                                                       |



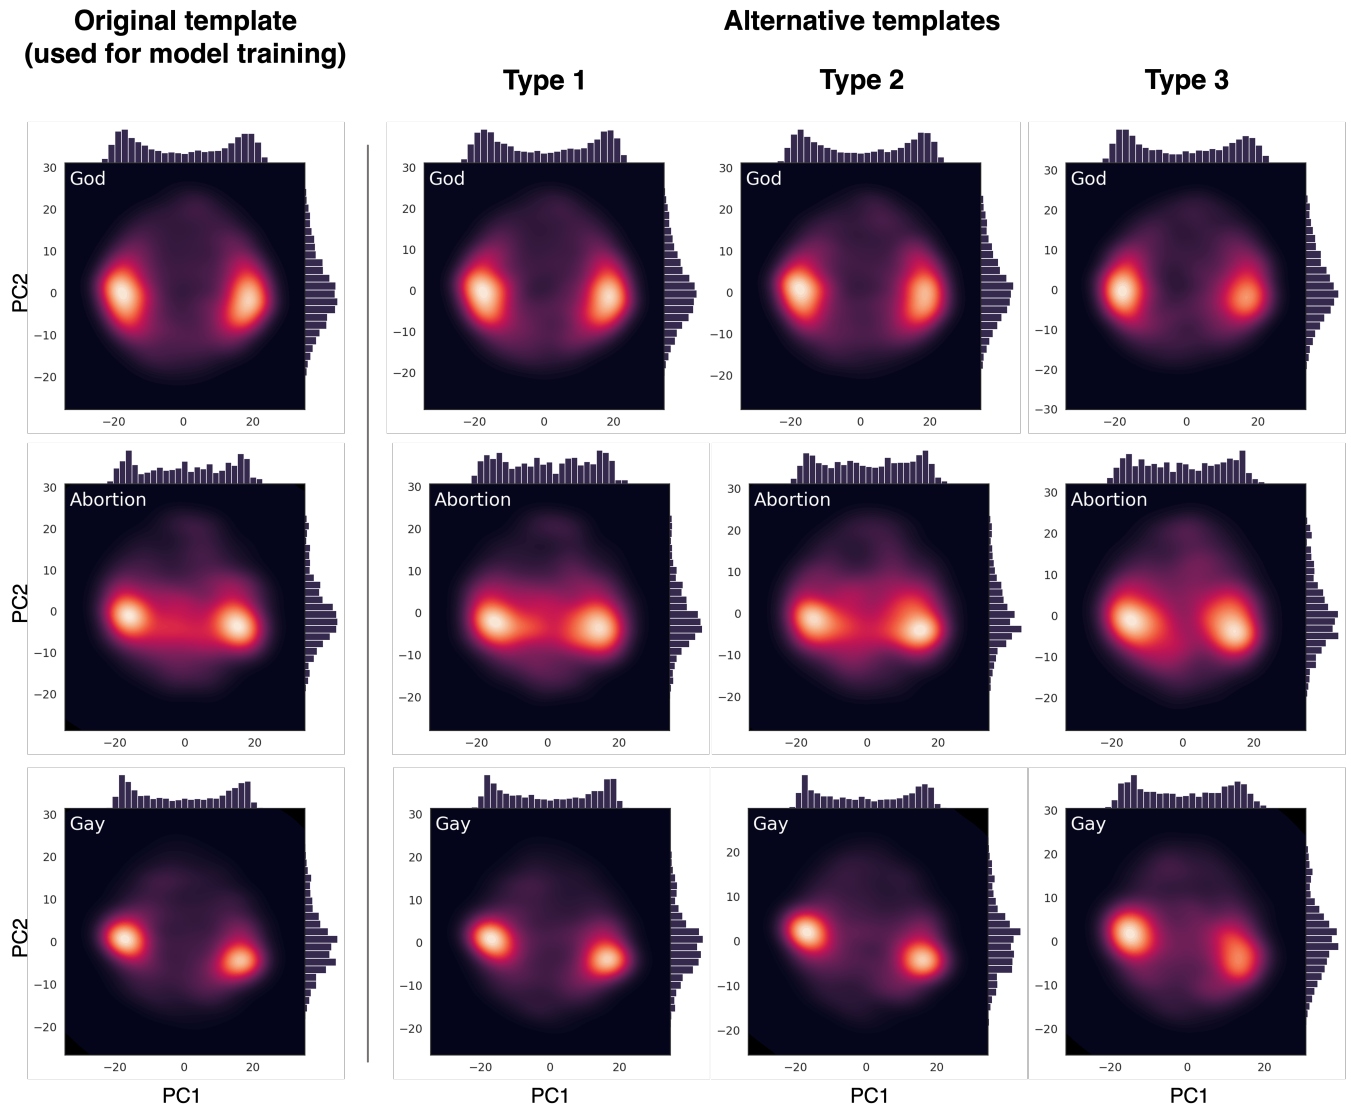

**Fig. S5.** The belief embeddings associated with three keywords ('God', 'Abortion', and 'Gay') are represented in the first two principal component (PC) spaces. The first column represents the belief embeddings generated using the original template ("I agree/disagree with the following: "). The other three columns represent the same belief set, but using the output vectors of beliefs rephrased with three alternative templates as shown in Table S2. The same model, which was fine-tuned using the beliefs with the original template, was used for generating the embeddings of rephrased beliefs. The PC space was calculated using the original belief embeddings. The bimodal shape of the belief distribution is preserved across different template choices.

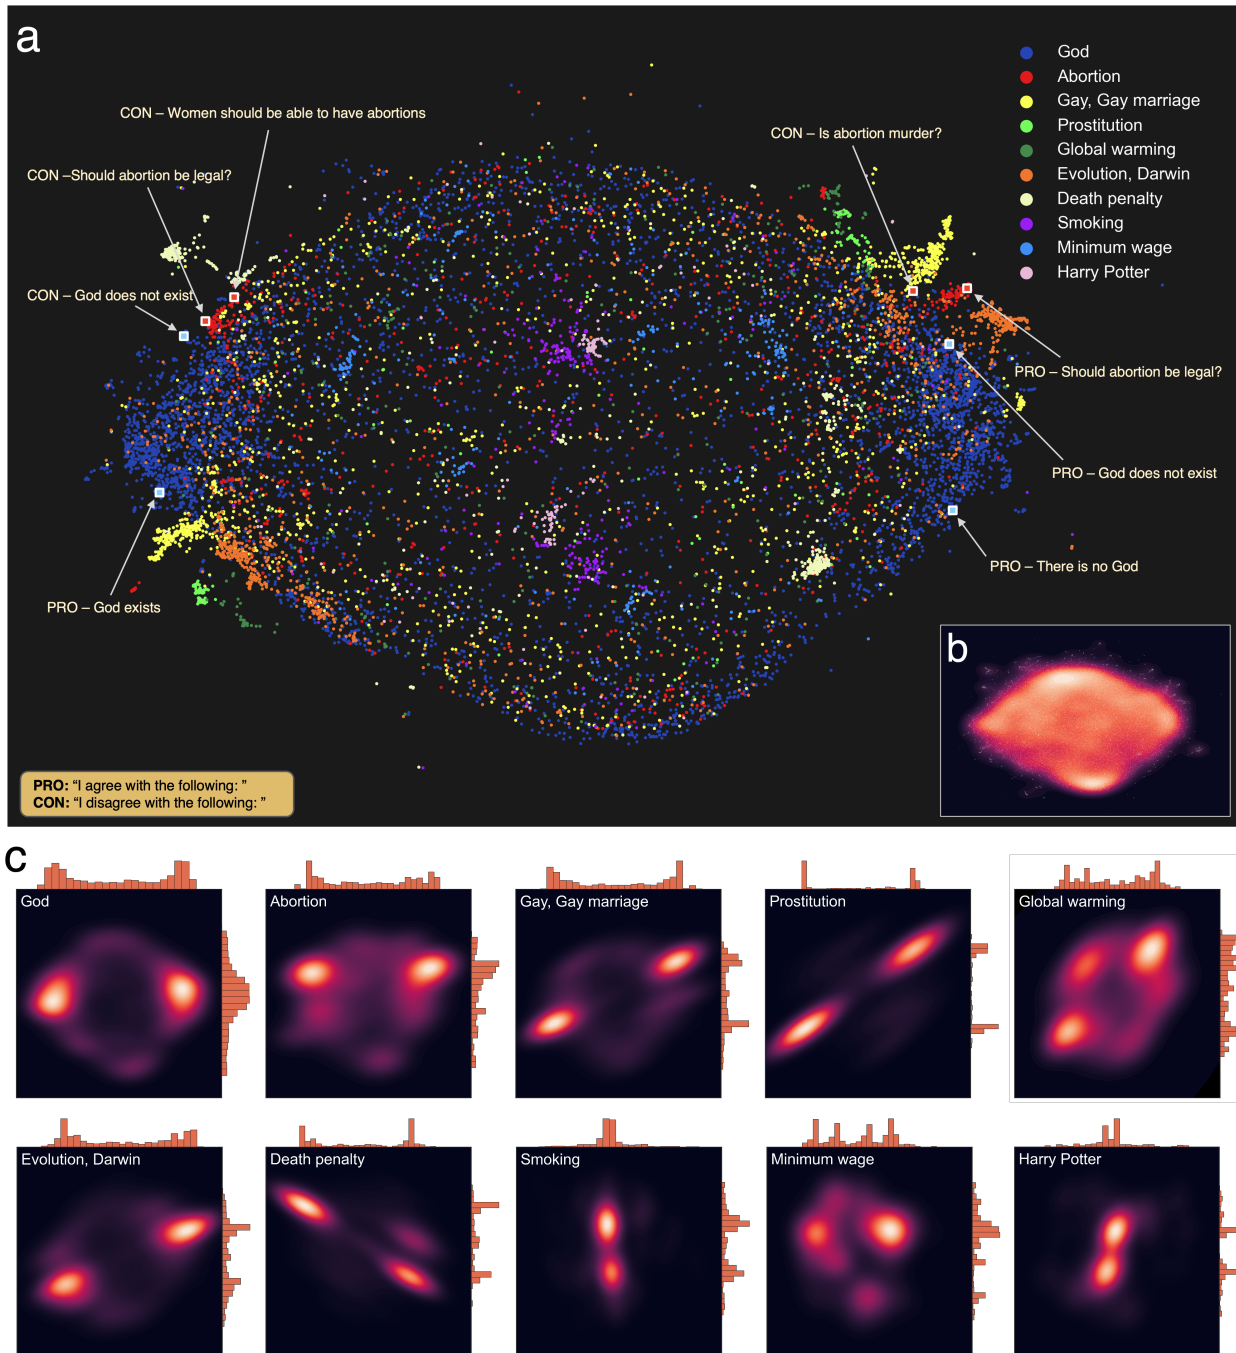

**Fig. S6.** The belief embeddings are projected into a 2-dimensional space using UMAP method. (a) Beliefs associated with 10 selected keywords are illustrated in different colors. The UMAP representation reveals that beliefs related to these keywords tend to form two meaningful clusters in the belief space. Representative examples from different belief clusters are depicted with accompanying text. (b) shows the UMAP representation of entire beliefs in the DDO dataset. The background heatmap, generated using a kernel density estimation method, indicates the density of beliefs, while the overlaid white dots represent individual beliefs. (c) demonstrates distributions of beliefs related to individual keywords in the UMAP space. Each belief distribution associated with different keywords reveals two highly clustered regions, spaced to varying degrees in different areas of the UMAP space. These patterns highlight the existence of polarization in beliefs related to various social issues.

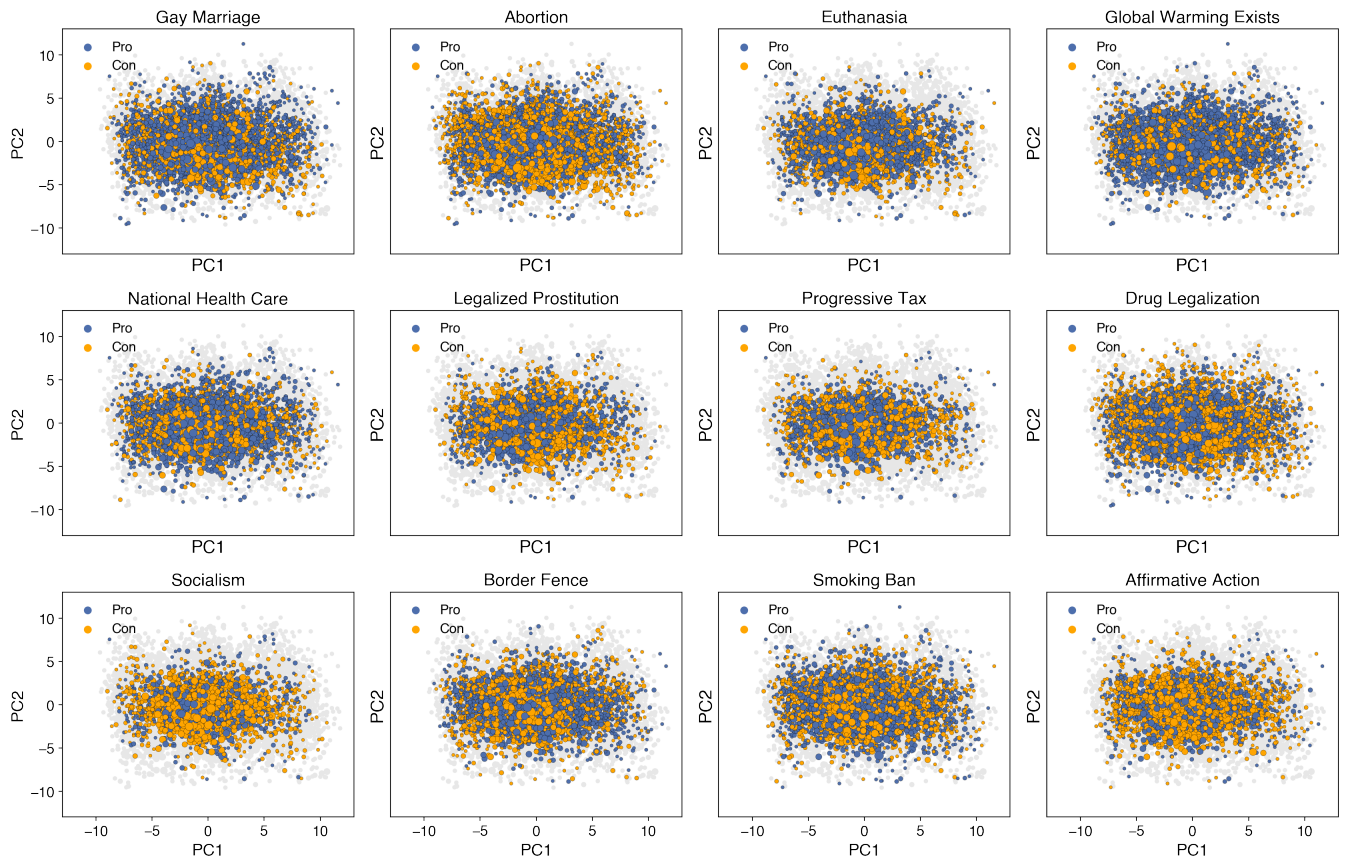

**Fig. S7.** Visualization of user embeddings in the belief space generated by the base S-BERT model before fine-tuning. Different user groups on various controversial social issues are depicted in distinct colors. While the fine-tuned model exhibits a clearer separation of two user groups in the belief space (Fig. 3 of the main manuscript), the user embeddings calculated by the base S-BERT model do not show such separation.

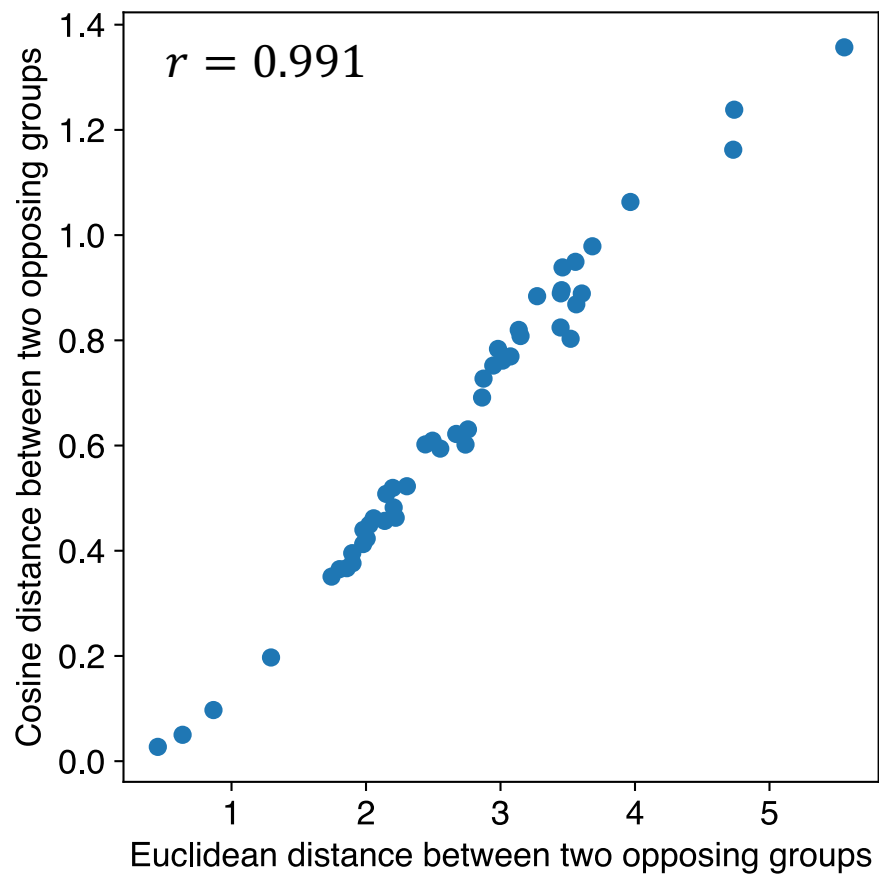

**Fig. S8.** Comparison of Euclidean and cosine distances between two user groups with opposing opinions on 48 major social issues. The two distance metrics are highly correlated, with Pearson correlation  $r = 0.991$ ,  $P < 0.001$ .

| Dataset index | # users | # debates (Train set) | # debates (Test set) | Average length of vote history per user (Train set) |
|---------------|---------|-----------------------|----------------------|-----------------------------------------------------|
| 1             | 10,173  | 42,255                | 11,581               | 10.98                                               |
| 2             | 10,401  | 42,464                | 11,571               | 10.66                                               |
| 3             | 9,706   | 40,936                | 11,720               | 11.04                                               |
| 4             | 9,675   | 42,409                | 11,327               | 11.74                                               |
| 5             | 9,744   | 41,591                | 11,682               | 11.31                                               |

**Table S4. Description of the train and test datasets used for the belief prediction task. A 5-fold evaluation is used for the binary classification of users' beliefs.**

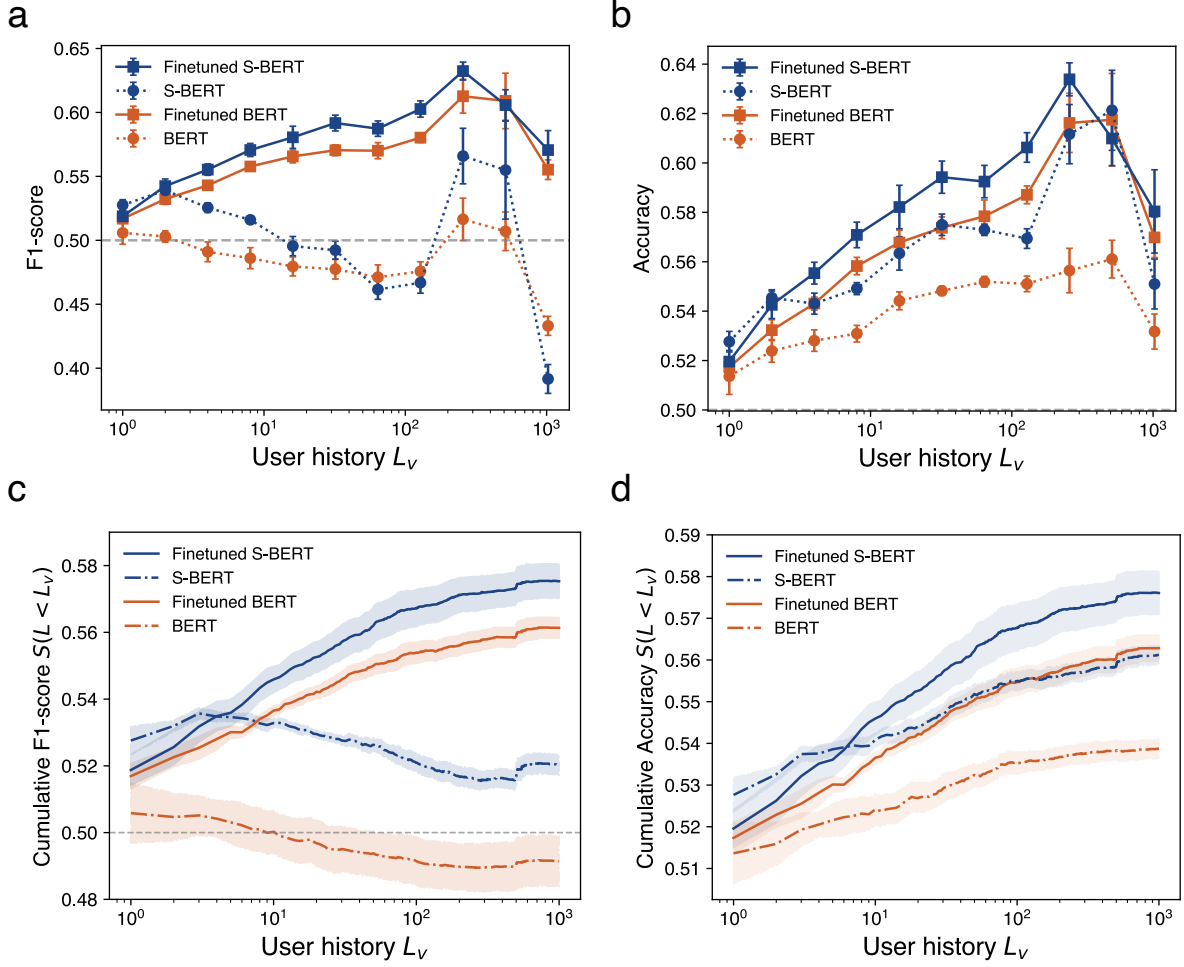

**Fig. S9.** Performance of belief prediction downstream task over the length of users' voting history  $L_v$ . (a) and (b) show the relation between F1-score and accuracy with  $L_v$ . (c) and (d) show the relationship between cumulative F1-score (accuracy)  $S(L < L_v)$  and  $L_v$ , where  $S(L < L_v)$  represents the F1-score (accuracy) for users with voting records shorter than  $L_v$ . User beliefs are more accurately predicted as more voting records are accumulated.

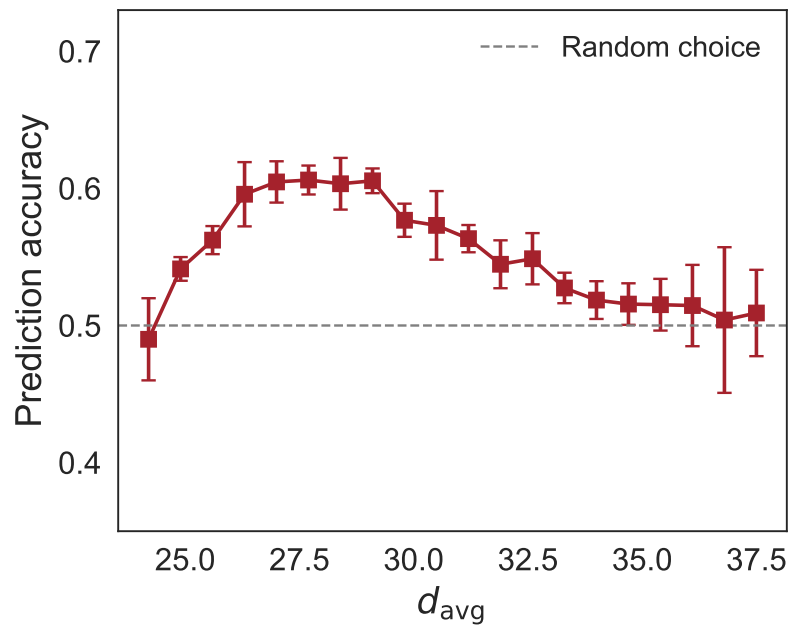

**Fig. S10.** Average accuracy for belief prediction task over the average distances  $d_{avg}$  of two contrasting beliefs from users.

## References

1. E Durmus, C Cardie, A corpus for modeling user and language effects in argumentation on online debating. *arXiv preprint arXiv:1906.11310* (2019).
2. E Durmus, C Cardie, Exploring the role of prior beliefs for argument persuasion. *arXiv preprint arXiv:1906.11301* (2019).
3. OpenAI, Gpt-4 (<https://openai.com>) (2023) Accessed: 2024-03-23.
4. L McInnes, J Healy, J Melville, Umap: Uniform manifold approximation and projection for dimension reduction. *arXiv preprint arXiv:1802.03426* (2018).
